# Supplementary material for: Confidence-Ranked Reconstruction of Census Microdata from Published Statistics
Source: arXiv:2211.03128 source file (2023-02-06)
Supplement: Supplementary file 1 [file supplement.tex]

%%% PNAS Supporting Information style file
%%% For use with pnas-new.cls
\NeedsTeXFormat{LaTeX2e}
\ProvidesPackage{pnassupportinginfo}[2022/07/12 v1.7 PNAS supporting information style]

%% Set whether the abstract is set into the first column
\setboolean{shortarticle}{true} 
% true = set into first column
% false = spans page width

%% Remove "DRAFT" watermark
\setboolean{displaywatermark}{false}

%% v1.5: new SI format is single column
\onecolumn

%% Set colors
\definecolor{color2}{RGB}{130,0,0} % color

%% keep the value of author for the footer
\RequirePackage{authoraftertitle}

\RequirePackage{totcount,xpatch}
\regtotcounter{section}
\regtotcounter{figure}
\regtotcounter{table}
\regtotcounter{NAT@ctr}  %% thanks to natbib

%% v1.5: New counters
\newtotcounter{movie}
\newtotcounter{dataset}

\newtotcounter{SItext}

% v1.7: Change all "Supplementary" to "Supporting"

%% v1.5: new title page format

\renewcommand{\@maketitle}{%
  \begin{center}
  \includegraphics[width=9.95cm]{pnas-logo}
  \end{center}
  \vskip45pt
  \begingroup
  \raggedright
  {\Huge\sffamily\bfseries Supporting Information for\par}
  \bigskip
  {\LARGE\sffamily\bfseries\@title\par}
  \bigskip
  {\@author\par\bigskip\@correspondingauthor\par}
  \endgroup
  \bigskip
  \section*{This PDF file includes:}
  \ifnum\numexpr\totvalue{SItext}+\totvalue{figure}+\totvalue{table}+\totvalue{movie}+\totvalue{dataset}+\totvalue{NAT@ctr}\relax > 0
    \begin{list}{}{%
    \setlength\leftmargin{2em}%
    \setlength\itemsep{0pt}%
    \setlength\parsep{0pt}}
    %% Check if there is some SI text
    \ifnum\totvalue{SItext}>0
      \item Supporting text
    \fi
    %% Total # of figures
    \ifnum\totvalue{figure}>0
      \item
      \ifnum\totvalue{figure}=1
       Fig.~S1 %(not allowed for Brief Reports)
      \else
      Figs.~S1 to S\total{figure} %(not allowed for Brief Reports)
       \fi
    \fi
    %% Total # of tables
    \ifnum\totvalue{table}>0
      \item
      \ifnum\totvalue{table}=1
     Table S1 %(not allowed for Brief Reports)
      \else
      Tables S1 to S\total{table} %(not allowed for Brief Reports)
       \fi
     \fi
    %%% Total # of movies
    \ifnum\totvalue{movie}>0
      \item
      \ifnum\totvalue{movie}=1
      Legend for Movie S1
      \else
      Legends for Movies S1 to S\total{movie}
      \fi
    \fi
    %%% Total # of datasets
    \ifnum\totvalue{dataset}>0
      \item
      \ifnum\totvalue{dataset}=1
      Legend for Dataset S1
      \else
      Legends for Dataset S1 to S\total{dataset}
      \fi
    \fi
    %%% Whether there's a references section
    \ifnum\totvalue{NAT@ctr}>0
      \item SI References
    \fi
  \end{list}
  \fi
  \ifnum\numexpr\totvalue{movie}+\totvalue{dataset}\relax > 0
  \section*{Other supporting materials for this manuscript include the following: }
  \begin{list}{}{%
  \setlength\leftmargin{2em}%
  \setlength\itemsep{0pt}%
  \setlength\parsep{0pt}}
  %%% Total # of movies
  \ifnum\totvalue{movie}>0
    \item
    \ifnum\totvalue{movie}=1
    Movie S1
    \else
    Movies S1 to S\total{movie}
    \fi
  \fi
  %%% Total # of datasets
  \ifnum\totvalue{dataset}>0
    \item
    \ifnum\totvalue{dataset}=1
    Dataset S1
    \else
    Datasets S1 to S\total{dataset}
    \fi
  \fi
  \end{list}
  \fi
  \clearpage
}

\additionalelement{}
\appto{\maketitle}{\thispagestyle{fancy}}

\fancyfoot[RO,LE]{\bfseries\sffamily\thepage\space of \pageref{LastPage}}
\fancyfoot[LO,RE]{\bfseries\sffamily\MyAuthor\space}

%% v1.5: Reset reference list settings

%% v1.5: Force floats to each occupy one page
\RequirePackage{float}
\RequirePackage{placeins}
\floatplacement{figure}{p}
\floatplacement{table}{p}

\setlength{\@fpsep}{\textheight}

%% v1.5 Typeset Movie and Dataset legends

\endinput
